# Supplementary material for: Macroscopic Spin-Orbit Interaction through Strong-Field Pumping of Inhomogeneously Aligned Molecular Ensemble
Source: arXiv:2602.09625 ancillary file (2026-07-14)
Supplement: Supplementary file 1 [file manuscript_SI.pdf]

# Macroscopic Spin-Orbit Interaction through Strong-Field Pumping of Inhomogeneously Aligned Molecular Ensemble
# Supplementary Material

Uriel Zanzuri*
*The Raymond and Beverly Sackler Faculty of Exact Sciences*
*Tel Aviv University, Tel Aviv 6997801, Israel*

Sharly Fleischer
*Physical Chemistry Department, Raymond and Beverly Sackler Faculty of Exact Sciences, Tel Aviv University, Tel Aviv 6997801, Israel*

Tamar Seideman
*Department of Chemistry, Northwestern University, Evanston, Illinois 60208, USA*

Eldad Yahel, Amir Natan,† and Alon Bahabad‡
*The School of Electrical Engineering, Tel Aviv University, Tel Aviv 6997801, Israel*
(Dated: February 9, 2026)

## I. Selection-rules based explanation for the main results of this work

The results in our work, especially those shown in Fig.4-5 in the main text, can be explained using an intuitive approach:

The discussed diatomic molecules break the spherical symmetry and therefore do not obey the selection rules for atoms, in addition, their angle relative to the field, leads to an orientation dependent phase delay in the response. As a first approximation we treat the molecules as an atom, obeying the selection rules of an atom, but with the orientation affected phase delay.

Hence, the molecule is treated as a point source obeying SAM conservation rule: $\sigma_q = n_1\sigma_1 + n_2\sigma_2$ [1] where $\sigma_q$ is the SAM of the emitted harmonic order $q$, $\sigma_{1,2}$ are the SAM of the two pump components (oscillating at the fundamental and second harmonic, respectively) and $n_1, n_2$ are the number of photons contributed by the two pump field components respectively. Together with energy conservation: $\omega_q = n_1\omega_1 + n_2\omega_2$ and limiting $\sigma_i = \pm 1$ $(i = 1, 2, q)$ $(\sigma = -1(1)$ for RHC(LHC)) we get the microscopic selection rules: $n_1 = n_2 \pm 1$ and $q = 3m \pm 1$, $m \in \mathbb{Z}$. Now, because we actually have a diatomic molecule, the response of the molecules would actually yield an elliptical polarization made of LHC and RHC components. The microscopically allowed component (for a point source) is assumed to be the dominant one - and it would be stronger than the other component and also locked in phase to the pump field with no dependence on the relative angle of the molecule with respect to the field. The other component (which is forbidden for a point source) would be weaker and would rotate with the molecule. This intuitive approach is backed with a rigorous calculation in section II below, showing that the polarizability of a rotated diatomic molecule subject to a circularly polarized field would yield an elliptical polarization with a component that is locked to the exciting field and a counter-rotating component which is locked to the angle of the molecule.

Let us examine, for example, the case of the $5^{th}$ harmonic. Due to the microscopic selection rules its SAM is $\sigma_5 = 1$ (LHC), and so this is the dominant component which is locked in phase regardless of the angle of rotation of the molecule. The RHC component is weaker and rotates with the alignment angle of the molecule - giving rise to OAM in the far field. As the molecule is homonuclear, the state of the emitted field should be symmetric upon a 180° rotation, thus the overall phase acquired after a full rotation would be $4\pi$ leading to OAM whose magnitude is 2. For the RHC field a molecule with an advanced rotation angle would lag in its response over a molecule at a smaller rotation angle - so the sign of the OAM in the far field would be negative. Overall, the result is OAM of -2 in the far field. Switching the helicity of the bichromatic drive would lead to the LHC field component in the far field to possess +2 OAM. Thus this system acts as a molecular q-plate (alas with a difference compared to regular q-plate based on bi-birefringence material where for the latter a change in the SAM value of the transmitted field is also observed).

---

* urielzanzuri@mail.tau.ac.il
† amirnatan@tauex.tau.ac.il
‡ alonb@tauex.tau.ac.il

## II. A Simple Model for the Linear Response of a Diatomic Molecule to a BCCP Field

In this section we provide a simple analytical model considering only the linear response of a diatomic molecule to a BCCP field. The purpose is to corroborate the qualitative nature of the results obtained from the full TDDFT numerical model. In particular, we want to verify with the simple model that the polarization state of the emitted radiation is dependent on the alignment of the molecule and the form of this dependence.

Consider an electric field $\boldsymbol{E}(t)$ with components $E_y(t)$ and $E_z(t)$ in the $y$-$z$ plane. The components are given by:

$$E_y(t) = E_0\Big(\cos(\omega_0 t) + \cos(2\omega_0 t)\Big)$$

$$E_z(t) = \begin{cases} E_0\Big(\sin(\omega_0 t) - \sin(2\omega_0 t)\Big) & \text{if rotation state is `bcp'}, \\ E_0\Big(-\sin(\omega_0 t) + \sin(2\omega_0 t)\Big) & \text{if rotation state is `bcm'}. \end{cases}$$

The polarizability tensor for $H_2^+$ is given by [2]:

$$\boldsymbol{\alpha} = \begin{pmatrix} 1.74 & 0 & 0 \\ 0 & 1.74 & 0 \\ 0 & 0 & 5.06 \end{pmatrix}.$$

The rotation matrix for an angle $\alpha$ in the $y$-$z$ plane is:

$$R(\alpha) = \begin{pmatrix} 1 & 0 & 0 \\ 0 & \cos(\alpha) & -\sin(\alpha) \\ 0 & \sin(\alpha) & \cos(\alpha) \end{pmatrix}.$$

The rotated polarizability tensor is then:

$$\boldsymbol{\alpha}' = R(\alpha)\boldsymbol{\alpha}R(\alpha)^T.$$

Working through the multiplication yields:

$$\boldsymbol{\alpha}' = \begin{pmatrix} 1.74 & 0 & 0 \\ 0 & 1.74\cos^2(\alpha) + 5.06\sin^2(\alpha) & (5.06 - 1.74)\sin(\alpha)\cos(\alpha) \\ 0 & (5.06 - 1.74)\sin(\alpha)\cos(\alpha) & 5.06\cos^2(\alpha) + 1.74\sin^2(\alpha) \end{pmatrix}.$$

For the BCP system the fields are:

$$E_y = E_0\Big[\cos(\omega_0 t) + \cos(2\omega_0 t)\Big], \qquad E_z = E_0\Big[\sin(\omega_0 t) - \sin(2\omega_0 t)\Big].$$

Their Fourier transforms are:

$$F[E_y] = \sqrt{\frac{\pi}{2}}\Big(\delta(\omega - \omega_0) + \delta(\omega + \omega_0) + \delta(\omega - 2\omega_0) + \delta(\omega + 2\omega_0)\Big),$$

$$F[E_z] = i\sqrt{\frac{\pi}{2}}\Big(\delta(\omega - \omega_0) - \delta(\omega + \omega_0) - \delta(\omega - 2\omega_0) + \delta(\omega + 2\omega_0)\Big).$$

The induced dipole moments after rotation are:

$$p'_y = \alpha'_{yy}E_y + \alpha'_{yz}E_z, \qquad p'_z = \alpha'_{zy}E_y + \alpha'_{zz}E_z.$$

Defining the left-hand and right-hand circular components as

$$p_{\text{LHS}} = \frac{p'_y + i\,p'_z}{\sqrt{2}}, \qquad p_{\text{RHS}} = \frac{p'_y - i\,p'_z}{\sqrt{2}},$$

their Fourier transforms are given by:

$$F[P_{\rm LHS}] = \frac{F[p'_y] + i\,F[p'_z]}{\sqrt{2}}, \qquad F[P_{\rm RHS}] = \frac{F[p'_y] - i\,F[p'_z]}{\sqrt{2}}.$$

After grouping terms, the coefficients for the fundamental and second harmonics for the left-hand component become:

$$C_\omega = \frac{\sqrt{\pi}}{2}\Big(\alpha'_{yy} + i\,\alpha'_{zy} + i\,\alpha'_{yz} - \alpha'_{zz}\Big),$$

$$C_{2\omega} = \frac{\sqrt{\pi}}{2}\Big(\alpha'_{yy} + i\,\alpha'_{zy} - i\,\alpha'_{yz} - \alpha'_{zz}\Big),$$

with similar expressions for the right-hand component.

Figure 1 shows the amplitude and phase of the first two harmonics of $H_2^+$ under the BCCP field (analytical calculation). As explained in the main text, the microscopically allowed component (for a point source) is assumed to be the dominant one - and it shows stronger than the other component and is also locked in phase to the pump field with no dependency on the relative rotation of the molecule. The other component (which is forbidden for a point source) is weaker and rotates with the molecule. Notice the qualitative similarity to our numerical simulation in figure 3 in the main text.

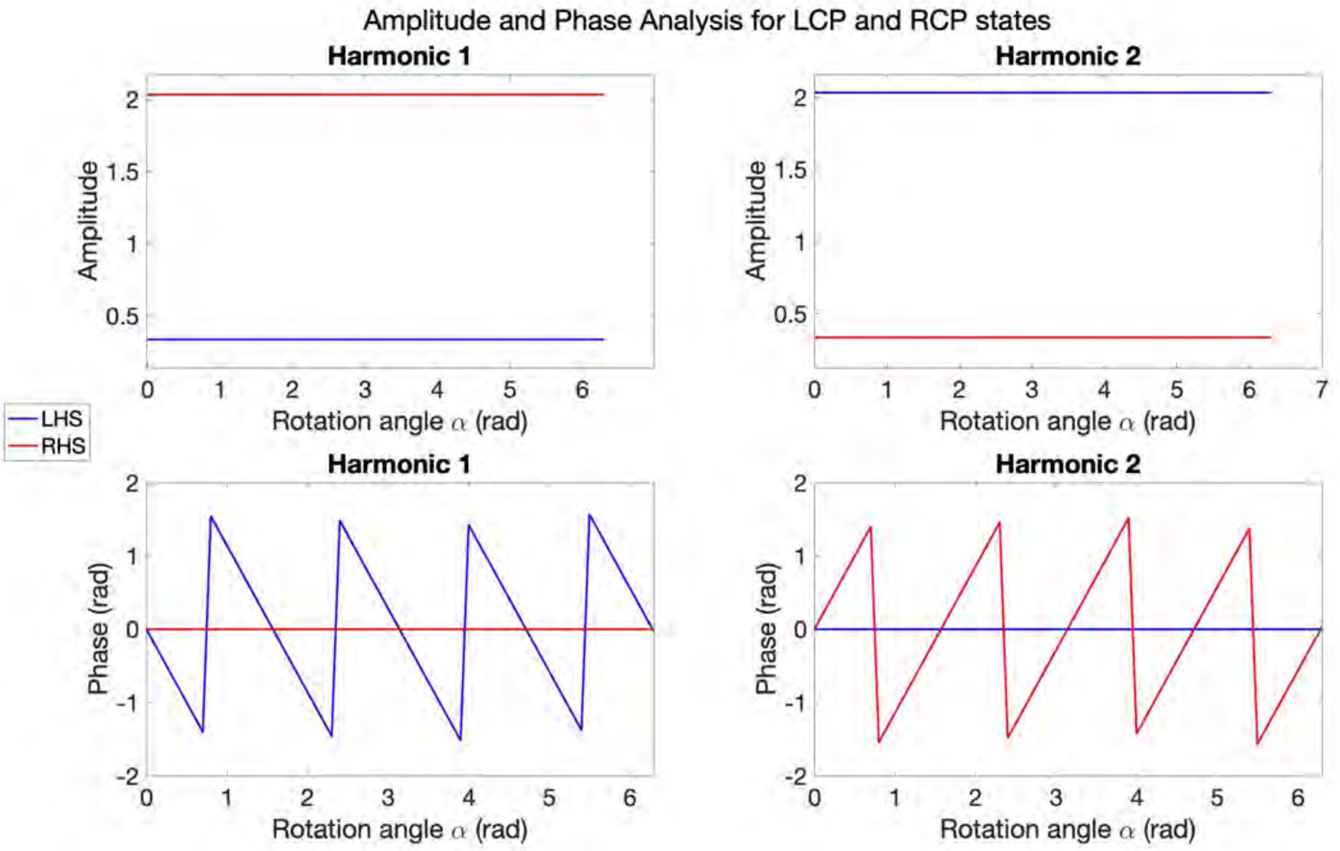


FIG. 1: Amplitude and phase of the first two harmonics of $H_2^+$ under a BCCP field (analytical calculation). The component forbidden for a point source is weaker but exhibits a phase that rotates linearly with the molecule's alignment angle

.

## III. TDDFT parameters

In this section we detail the simulation parameters for the RTTDDFT microscopic simulation used in our study. The computational domain was set to 40 atomic units with a grid resolution of $\Delta x = \Delta y = \Delta z = 0.4$ a.u. An absorbing layer of 5 a.u. with a damping exponent of 0.08 was applied to avoid reflections. The temporal resolution was 0.001 fs, ensuring stable propagation of the orbitals. Laser parameters include an amplitude of $3 \times 10^{14}$ W/cm$^2$, frequencies of $\omega_0 = 3.75 \times 10^{14}$ Hz and $2\omega_0$, and a pulse duration of 53.37 fs (approximately 20 optical cycles of the fundamental frequency). The laser pulse was shaped with a $\sin^2$ envelope. Tests we made indicated that a damping exponent of 0.08 provided clear, physical harmonic signals.

## IV. Additional Results

In this section, we extend our analysis of harmonic generation to a broader range of harmonics. In Subsection IV A, we present the calculated ellipticity and helicity for the first 25 harmonics (see Fig. 2 in the main text). In Subsections IV C and IV D, we explore the dependence of peak harmonics on the angle between the molecule and the field for $H_2^+$ and $N_2$, respectively.

### A. Ellipticity Values

| Harmonic Order | Ellipticity | Helicity |
|---|---|---|
| 1 | 0.37 | + |
| 2 | 0.36 | - |
| 3 | 0.19 | + |
| 4 | 0.44 | + |
| 5 | 0.70 | - |
| 6 | 0.17 | + |
| 7 | 0.15 | + |
| 8 | 0.19 | + |
| 9 | 0.18 | - |
| 10 | 0.10 | - |
| 11 | 0.15 | + |
| 12 | 0.03 | - |
| 13 | 0.06 | + |
| 14 | 0.03 | - |
| 15 | 0.03 | - |
| 16 | 0.08 | + |
| 17 | 0.06 | - |
| 18 | 0.03 | - |
| 19 | 0.08 | + |
| 20 | 0.02 | - |
| 21 | 0.14 | - |
| 22 | 0.05 | - |
| 23 | 0.12 | + |
| 24 | 0.16 | - |
| 25 | 0.23 | - |

TABLE I: Ellipticity (absolute values) and helicity for the first 25 harmonics in $H_2^+$.

### B. HHG spectrum — $N_2$

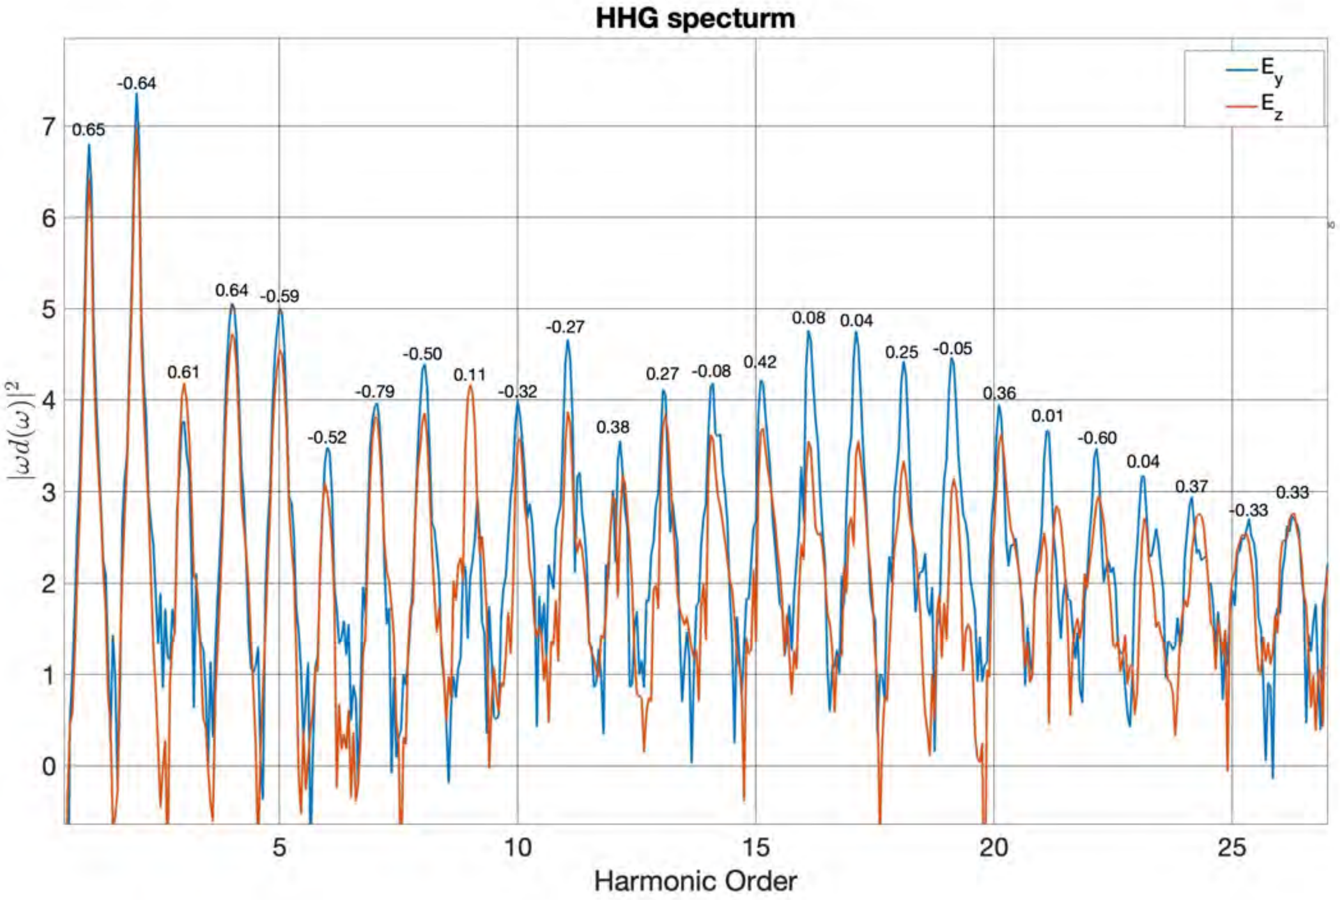


FIG. 2: Harmonic spectra for $\theta$ =0-degrees rotation of $N_2$ under a bi-chromatic laser field. The ellipticity for each harmonic order is shown above the peaks, the sign of which represents the handedness of the field. The appearance of both even and odd harmonics demonstrates the symmetry breaking induced by the counter-rotating bi-chromatic field.

### C. Amplitude and Phase — $N_2$

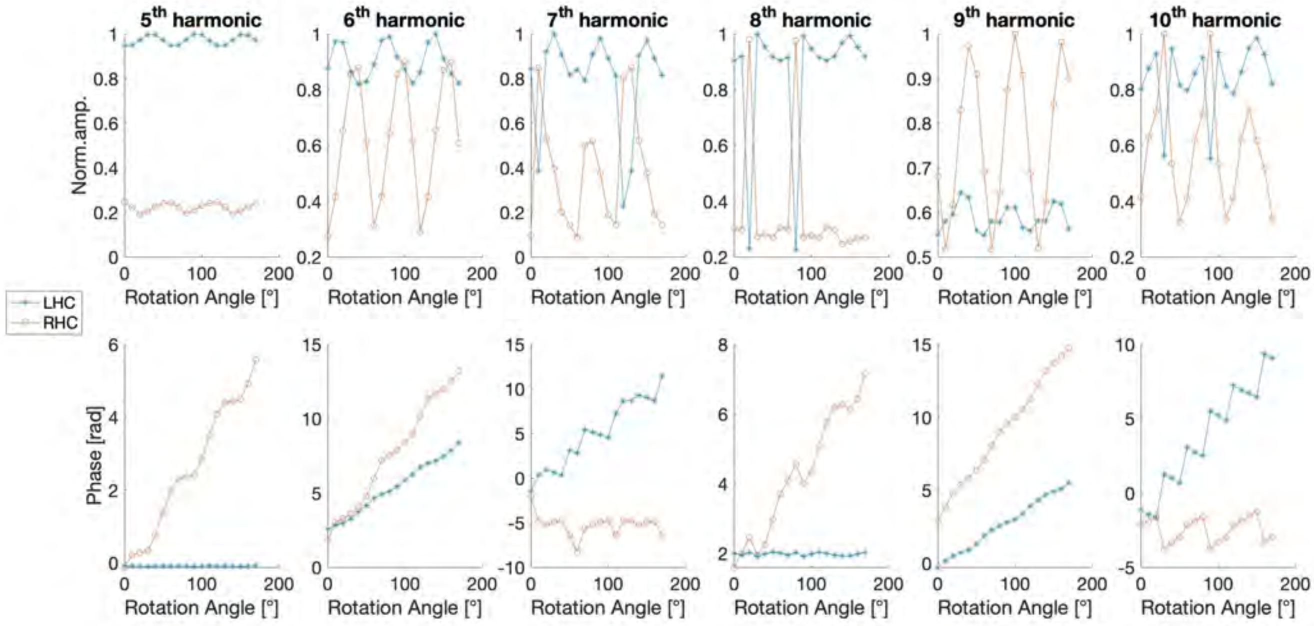


FIG. 3: Amplitude and phase of the $5^{th}$ to $10^{th}$ harmonics of a $N_2$ molecule under a clockwise BCCP polarized laser field. The linear dependence of the phase on the alignment angle observed for certain harmonic orders is the crucial microscopic requirement for generating integer OAM values in the macroscopic far-field radiation.

### D. Amplitude and Phase — $H_2^+$

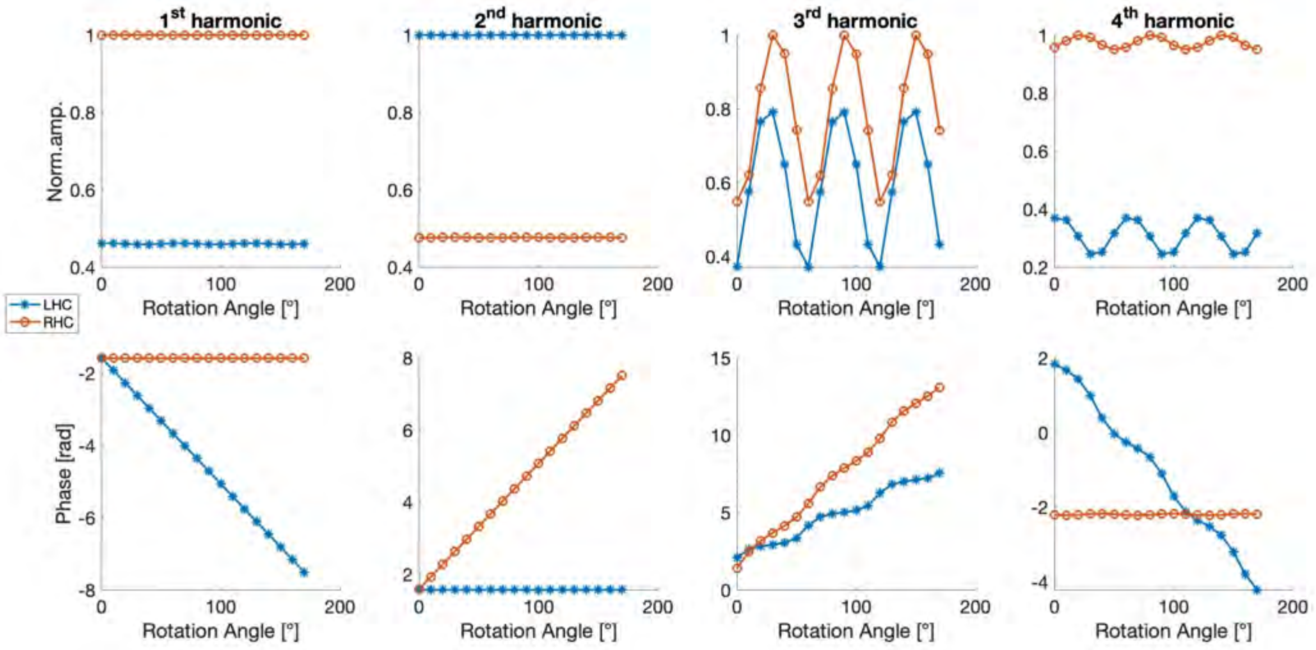


FIG. 4: Amplitude and phase of the $1^{st}$ to $4^{th}$ harmonics of a $H_2^+$ molecule under a clockwise BCCP laser field. The linear dependence of the phase on the alignment angle observed for certain harmonic orders is the crucial microscopic requirement for generating integer OAM values in the macroscopic far-field radiation

## V. $H_2^+$ Far-Field Patterns

In this section, we present far-field phase and intensity patterns alongside an approximate restoration of the field using dominant Laguerre-Gaussian (LG) modes for $H_2^+$ oriented molecules under different pump laser fields. In the figures below, the upper row shows the far-field pattern achieved from the simulation while the lower row shows the reconstructions of the field from the first 45 LG modes of the original field. The left and right panels in each figure show the left and right components of the field. Below each figure shows the far-field patterns we added a heat map that holds the relative weight of each LG mode. The decomposition involved projecting the field onto the modes, spanning azimuthal indices $l = -4$ to $l = 4$ and radial indices $p = 0$ to $p = 4$. The decomposition to LG modes allows us to see what OAM is related to the field. The first sub-section shows the results of the first harmonic far-field pattern generated in the case of a linearly polarized laser field. As was expected we see that the field holds zero orbital angular momentum. In the second and third sub-sections, we show the results of the fourth and fifth harmonics under the clockwise BCCP field and counter-clockwise field respectively. We see that the setting of the BCCP pump field gives rise to macroscopic spin-orbit interaction where High Harmonic radiation is emitted while imbued with Orbital Angular Momentum (OAM) whose sign is dependent on the helicity of the pump field. The effect of controlling the OAM sign can easily be seen in the decomposition heat map, we see a clear "role switching" between the left and right circular components of the far field when changing the circularity of the left and right circular field components of the laser. For the fourth harmonic for example, we see dominant $l = 2$ for the left circular component and $l = 0$ for the right component under clockwise BCCP while $l = 0$ for the left circular component and $l = -2$ for the right component under counter-clockwise BCCP.

### A. Linearly Polarized Bi-Chromatic Laser Field — $1^{st}$ Harmonic

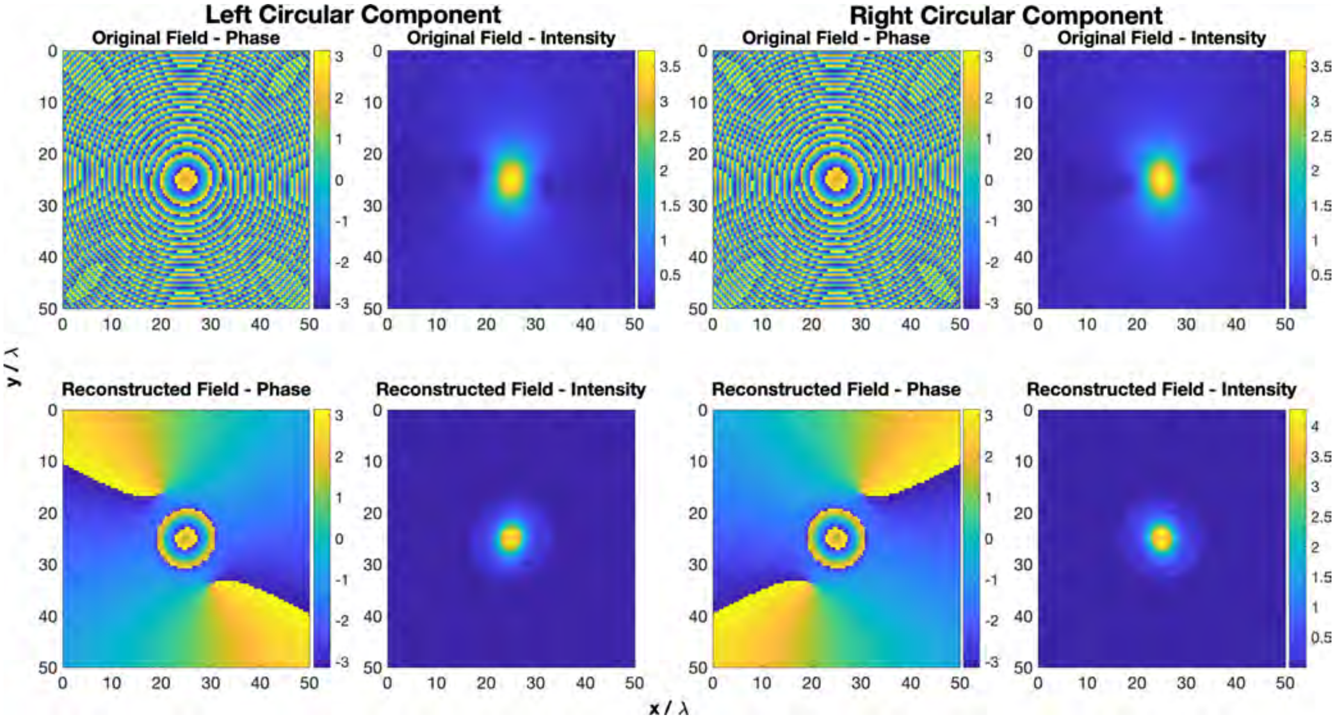


FIG. 5: Far-field pattern of the $1^{st}$ harmonic - a linearly polarized pump laser field. No signatures of OAM are observed in this case.

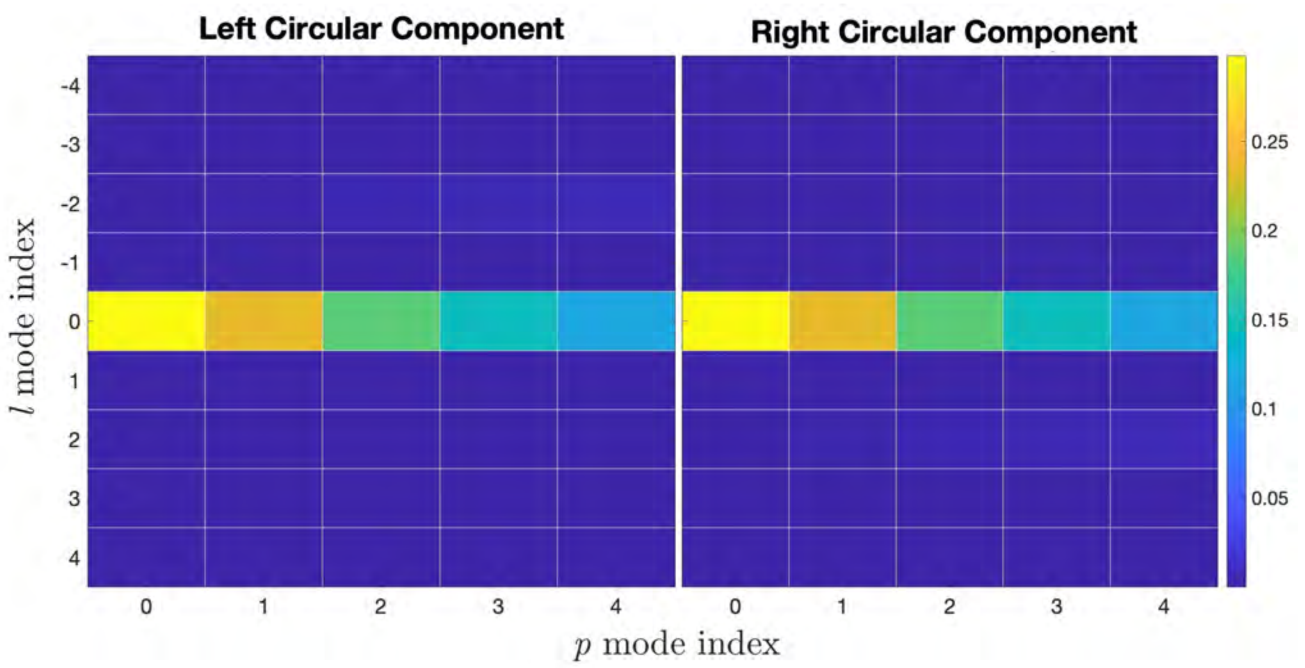


FIG. 6: LG-mode decomposition of the $1^{st}$ harmonic field - a linearly polarized pump laser field. The decomposition shows that no OAM is generated when the pump field lacks Spin Angular Momentum (SAM).

### B. Clockwise BCCP Field

*$4^{th}$ Harmonic*

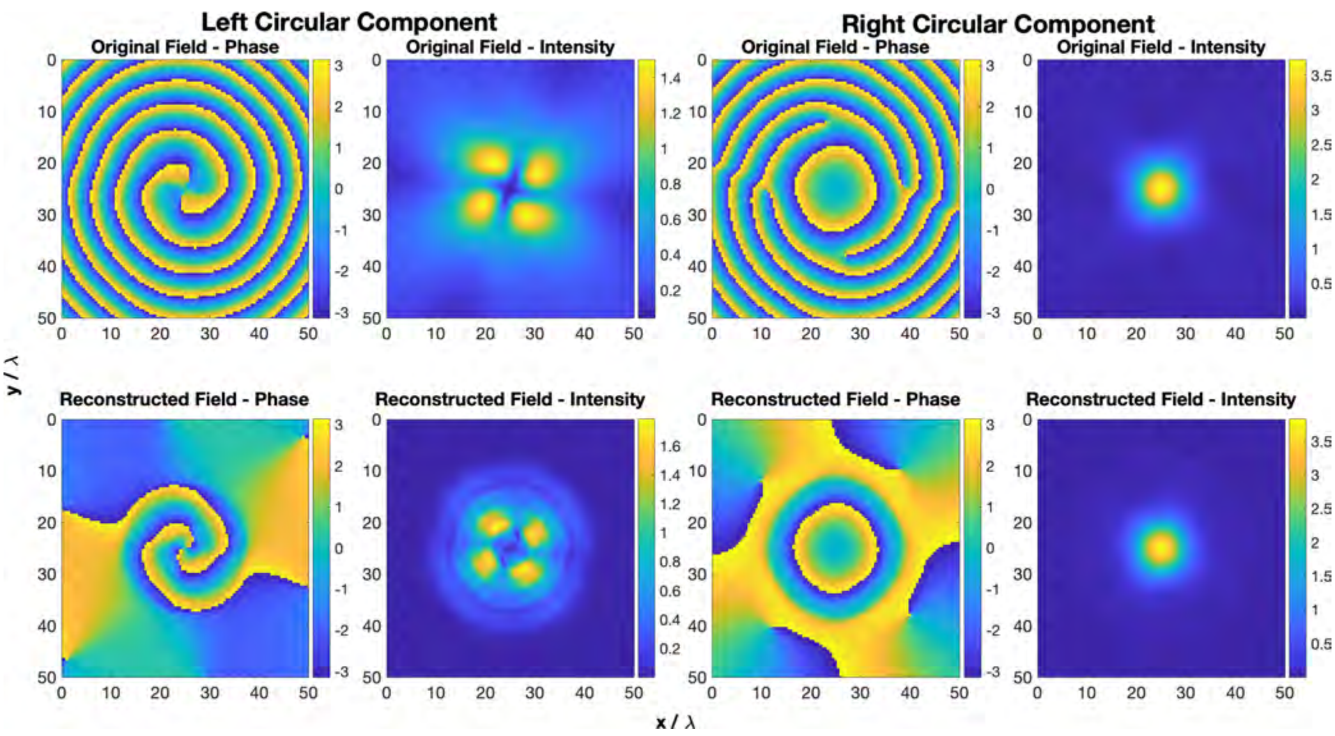


FIG. 7: Far-field pattern of the $4^{th}$ harmonic - a clockwise BCCP pump laser field. The left circular components shows OAM signature.

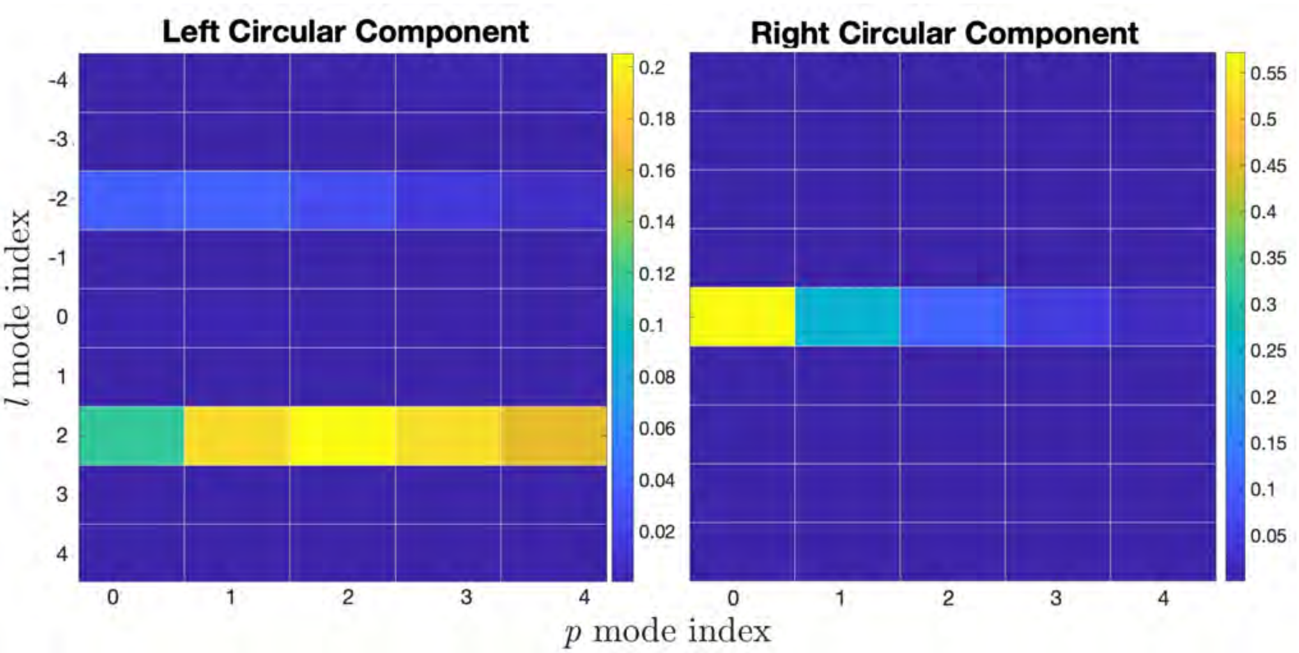


FIG. 8: LG-mode decomposition of the far-field pattern of the $4^{th}$ harmonic - a clockwise BCCP pump laser field. The decomposition shows that the Left Circular Component (LHC) carries dominant OAM l=+2, while the Right Circular Component (RHC) carries no OAM.

*$5^{th}$ Harmonic*

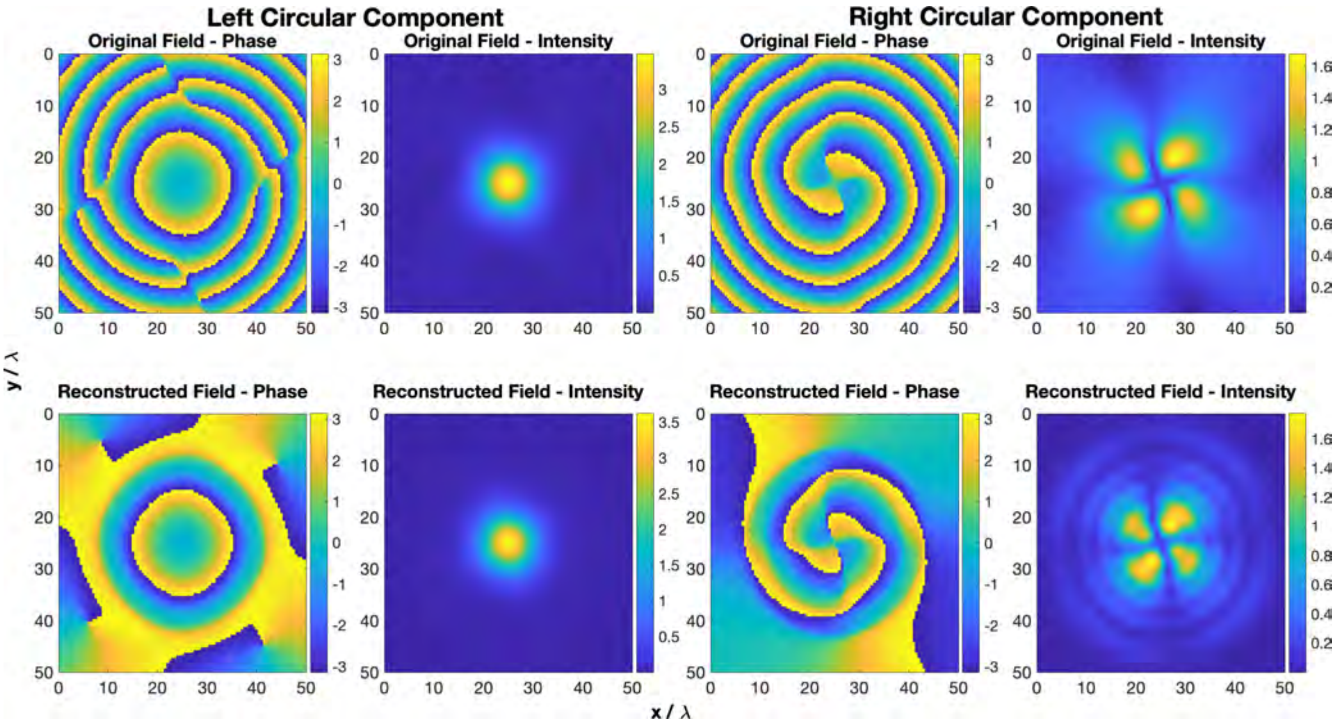


FIG. 9: Far-field pattern of the $5^{th}$ harmonic - a clockwise BCCP pump laser field. The right circular components shows OAM signature.

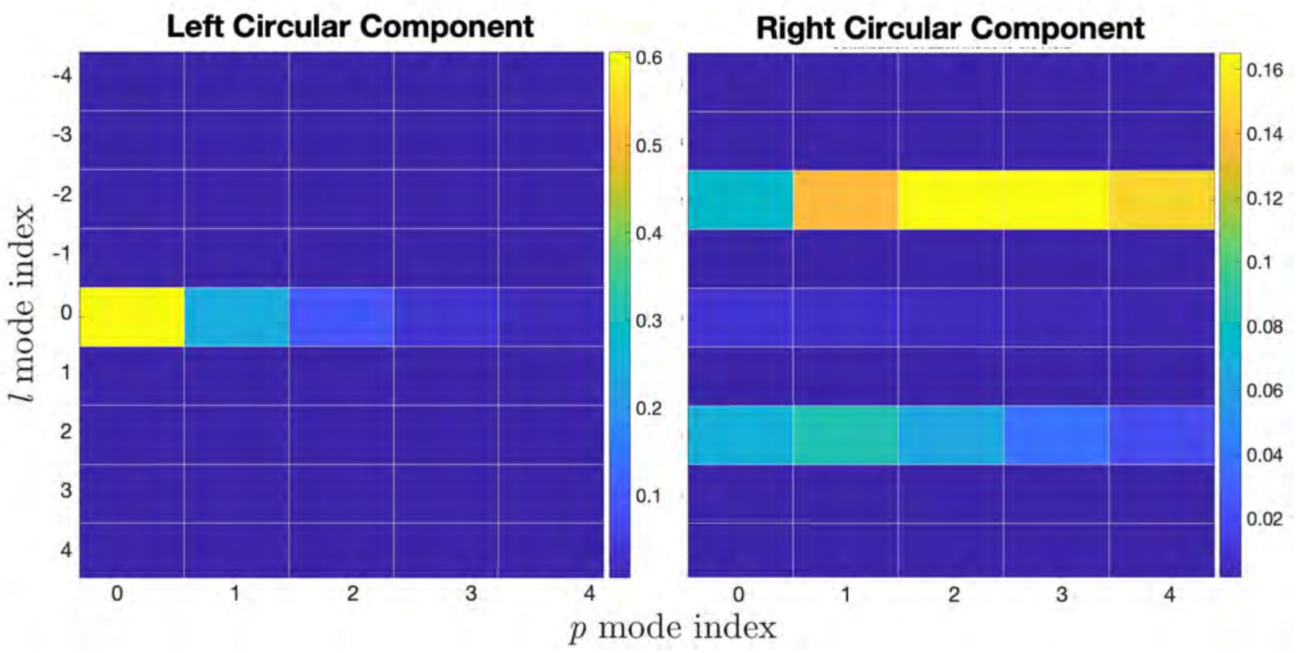


FIG. 10: LG-mode decomposition of the far-field pattern of the $5^{th}$ harmonic - a clockwise BCCP pump laser field. The composition shows that the right circular component carries dominant OAM l=-2.

### C. Counter-Clockwise BCCP Field

*$4^{th}$ Harmonic*

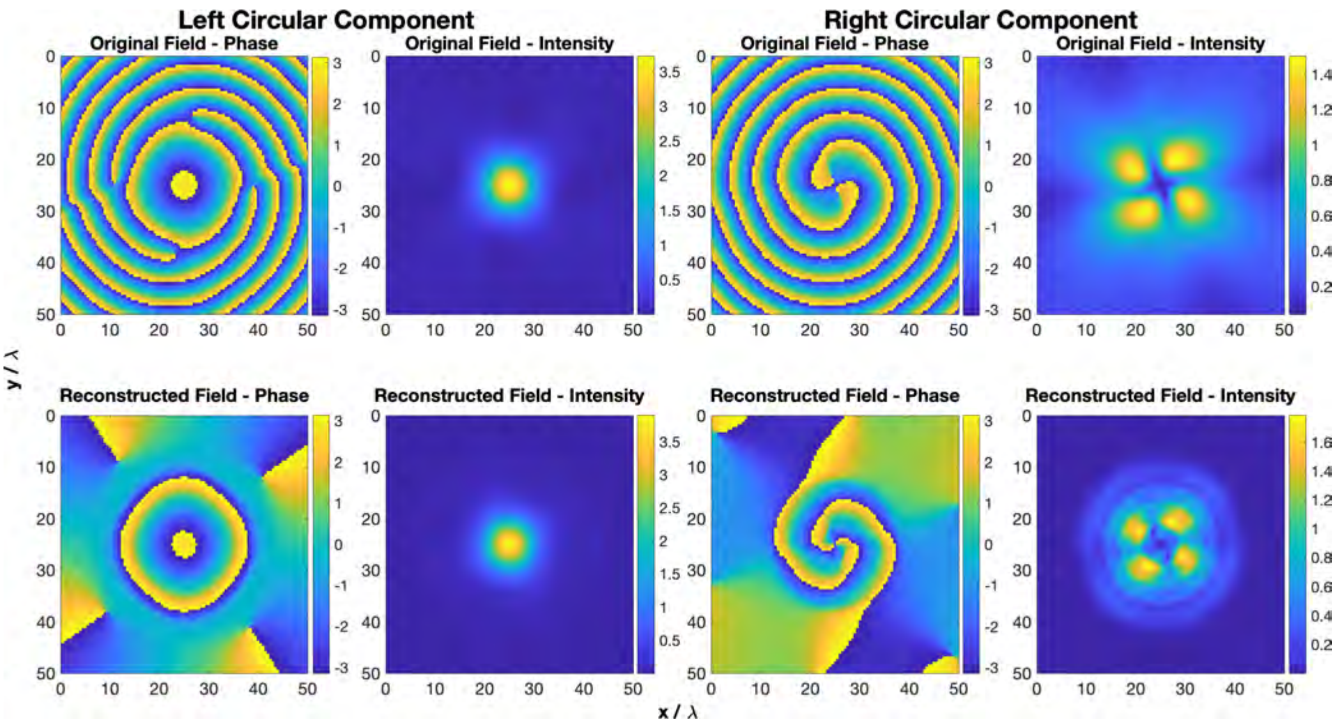


FIG. 11: Far-field pattern of the $4^{th}$ harmonic - a counter-clockwise BCCP pump laser field. The right circular components shows OAM signature.

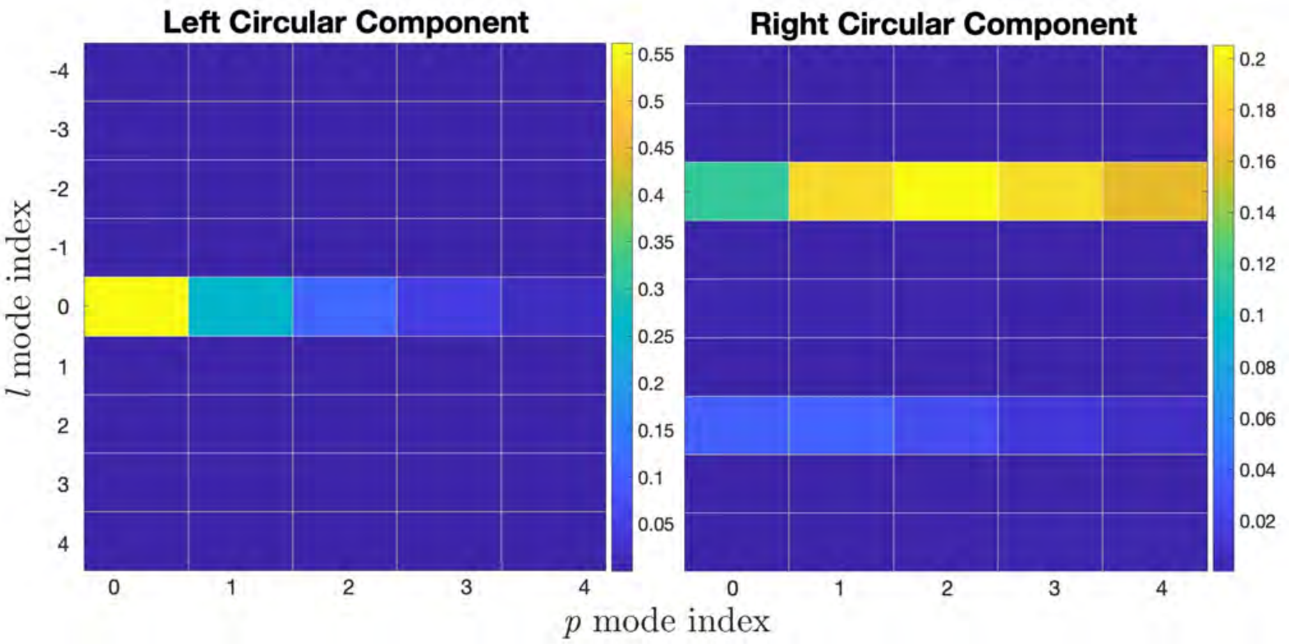


FIG. 12: LG-mode decomposition of the far-field pattern of the $4^{th}$ harmonic - a counter-clockwise BCCP pump laser field. The composition shows that the right circular component carries dominant OAM l=-2

.

*$5^{th}$ Harmonic*

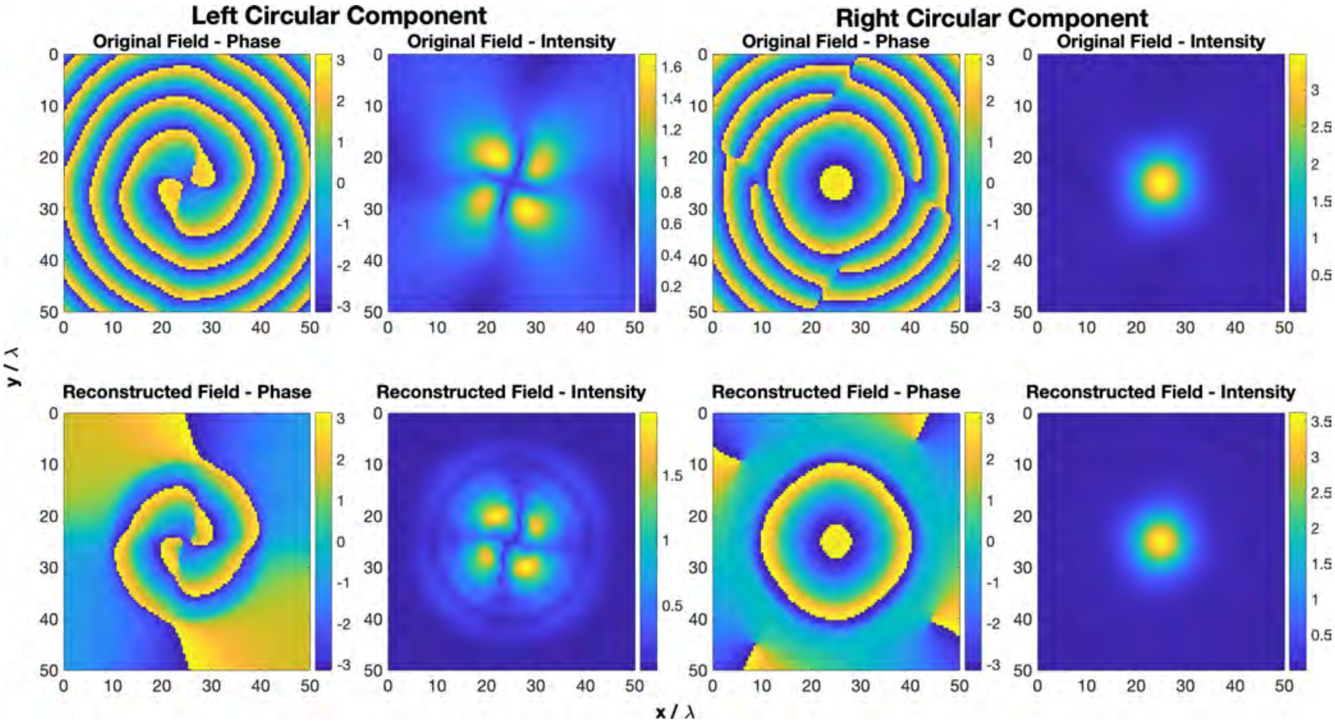


FIG. 13: Far-field pattern of the $5^{th}$ harmonic - a counter-clockwise BCCP pump laser field. The left circular components shows OAM signature.

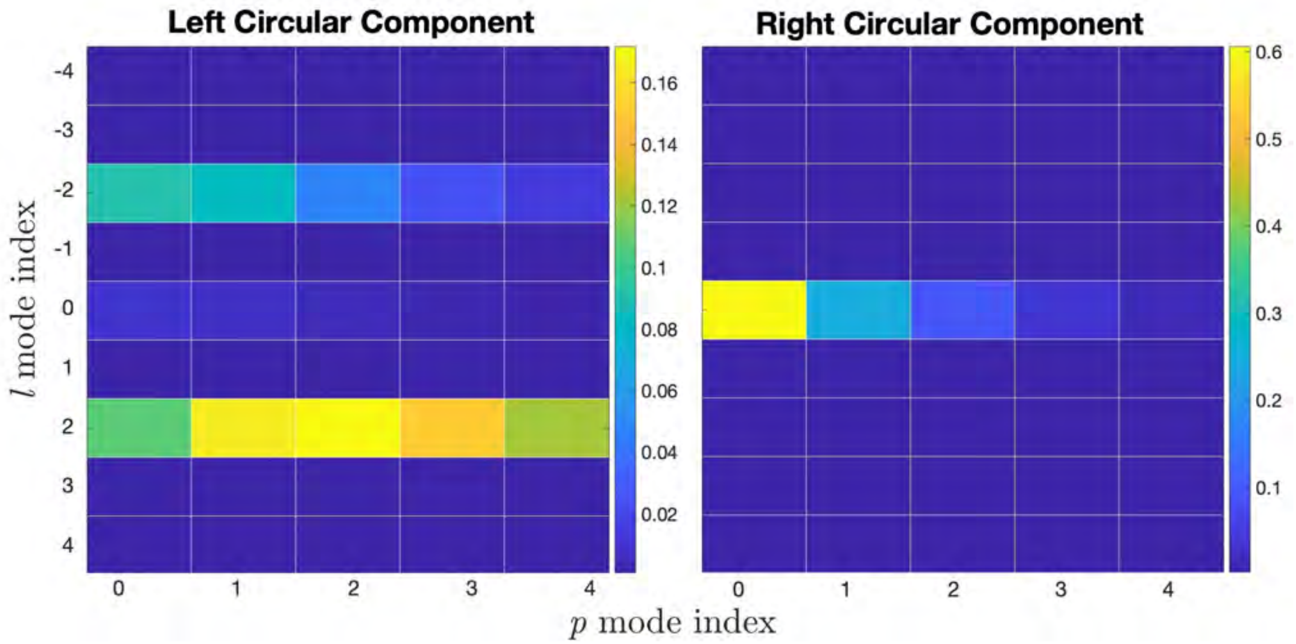


FIG. 14: LG-mode decomposition of the far-field pattern of the $5^{th}$ harmonic - a counter-clockwise BCCP pump laser field. The composition shows that the left circular component carries dominant OAM l=+2.

[1] A. Fleischer, O. Kfir, T. Diskin, P. Sidorenko, and O. Cohen, Spin angular momentum and tunable polarization in high-harmonic generation, Nature Photonics **8**, 543 (2014).

[2] D. Russell and I. I. I. Johnson, Nist computational chemistry comparison and benchmark database, NIST Standard Reference Database Number 101 (2022), accessed on November 25, 2024, Release 22.
